# Supplementary material for: Fast low-temperature irradiation creep driven by athermal defect dynamics
Source: arXiv:2401.13385 ancillary file (2024-01-24)
Supplement: Supplementary file 1 [file supplemental.pdf]

# ∾ Supplemental Material ∾

# Fast low-temperature irradiation creep driven by athermal defect dynamics

Alexander Feichtmayer,[1,2] Max Boleininger,[3,*] Johann Riesch,[1]
Daniel R. Mason,[3] Luca Reali,[3] Till Höschen,[1] Maximilian Fuhr,[1,2]
Thomas Schwarz-Selinger,[1] Rudolf Neu,[1,2] and Sergei L. Dudarev[3]

[1]*Max Planck Institute for Plasma Physics, Boltzmannstr. 2, 85748 Garching, Germany*
[2]*Technical University Munich, Boltzmannstr. 15, 85748 Garching, Germany*
[3]*UK Atomic Energy Authority, Culham Centre for Fusion Energy, Oxfordshire OX14 3DB, United Kingdom*

(Dated: January 24, 2024)

## CONTENTS

S1. Supplemental information to simulations 2
- A. SRIM recoil spectrum and dose profile 2
- B. Atomistic high-dose cascade simulations 3
- C. Estimating the wire temperature due to beam heating 6

S2. Supplemental information to experiments 9
- A. Sample material 9
- B. The GIRAFFE Experiment 11
- C. Irradiation-induced stress relaxation 12

References 14

## S1. SUPPLEMENTAL INFORMATION TO SIMULATIONS

### A. SRIM recoil spectrum and dose profile

The SRIM-2008[1] software, available online at http://www.srim.org/, is used to generate the atomic recoil spectrum and the dose profile. We run SRIM in the "Ion Distribution and Quick Calculation of Damage" mode[2,3], for $W^{6+}$ ions with 20.3 MeV energy impacting bulk tungsten. The primary recoil events are exported to the COLLISIONS.TXT file, which contains the coordinates and recoil energies of each event. We ran two SRIM simulations, one for $10^5$ ions using a threshold displacement energy of $E_\mathrm{d} = 90\,\mathrm{eV}$[4] for computing the damage profile after the NRT model[5], and the other for $10^4$ ions using $E_\mathrm{d} = 25\,\mathrm{eV}$ for the purpose of including statistics of damage-generating events above the minimum threshold energy $E_\mathrm{d}^\mathrm{min} = (41 \pm 8)\,\mathrm{eV}$[4], or 46 eV in the empirical tungsten potential by Mason *et al.*[6]. The former simulation is used to construct the dose profile, and the latter simulation is used to initiate collision cascades in the molecular dynamics simulations, see Sec. S1 B.

In SRIM, the surface lies normal to the x-direction, with ions approaching the surface along x-direction and impacting the surface at $(0, 0, 0)$. The spatial distribution of recoil events resembles a plume, spreading out towards x-direction from the origin, as pictured in Fig. S1a.

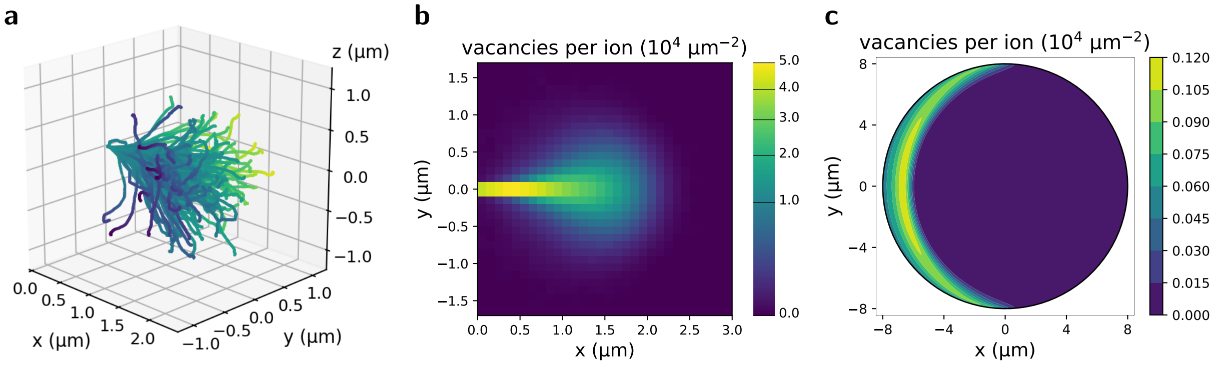


**Fig. S1: Generating the dose profile. a,** SRIM is used to generate a spatial map of primary recoil events generated by 20.3 MeV $W^{6+}$ ions impacting a tungsten foil at coordinate $(0, 0, 0)$, Only 2 % of all recoils are shown to visualise the ion paths, coloured by y-coordinate. **b,** The primary recoil energies are converted into the number of generated vacancies in accordance the NRT damage model, flattened along z-coordinate, binned, and interpolated to generate a vacancy density $\phi(x, y)$. **c,** The vacancy density $\phi(x, y)$ is convolved over the semi-circle representing the irradiated wire circumference to obtain the vacancy profile in the wire cross section.

Next, the recoil energies $E_\mathrm{R}$ are converted to damage energies $T_\mathrm{d}(E_\mathrm{R})$ following the Lindhard model[5], from which the number of vacancies $N_\mathrm{d}(T_\mathrm{d})$ generated per ion is computed using the NRT damage model[5] ($E_\mathrm{d} = 90\,\mathrm{eV}$). The recoil events are flattened along z-direction, binned into a histogram, and interpolated to obtain the distribution of vacancies generated per ion $\rho(x, y)$ shown in Fig. S1b. As the wire is thin ($\mathrm{R} = 8\,\mu\mathrm{m}$) compared to the beam spot width ($\mathrm{FWHM} \sim 1\,\mathrm{mm}$), we assume that the tungsten ions impact the wire with a uniform flux across its breadth. The distribution of vacancies generated per ion in

the wire cross-section is hence obtained by averaging across the wire semi-circle:

$$\rho_{\rm wire}(x,y) = \begin{cases} \dfrac{1}{2R}\displaystyle\int_{-R}^{R} {\rm d}s\, \rho(x-\sqrt{R^2-s^2}, y-s) & x^2+y^2 \le R^2 \\ 0 & \text{otherwise} \end{cases} \tag{S1}$$

The resulting profile is shown in Fig. S1c.

The damage profile can be converted into a dose-rate profile via

$$\dot\phi(x,y) = \rho_{\rm wire}(x,y)\frac{F(t)}{l_{\rm irr}\eta}, \tag{S2}$$

where $F(t)$ is the total ion flux impacting the wire, $l_{\rm irr}$ is the length of the irradiated wire section, and $\eta$ is the atomic number density. This conversion is not necessary for the purpose of solving the finite-element model; we are evolving the virtual wire simulation in the dose coordinate, rather than the time coordinate, and thus increment the dose profile by a fraction of the normalised damage profile.

### B. Atomistic high-dose cascade simulations

The cascade simulation procedure broadly follows the approach outlined in previous work[6]. The atomistic simulations here are intended to describe self-ion-irradiation of tungsten with 20.3 MeV ions under an externally applied uniaxial stress. The collision cascade simulations are performed under the constraint of maintaining a uniaxial stress of $\sigma_{\rm zz}^{\rm ext}$ on the simulation cell, with all other stress components set to zero. The simulation cell is spanned by the unit vectors $\hat{\boldsymbol{c}}_x = [100]$, $\hat{\boldsymbol{c}}_y = [010]$, and $\hat{\boldsymbol{c}}_z = [001]$, with crystal unit cells following the same orientation.

The defect content at high dose strongly depends on the recoil energy spectrum[6]. To ensure consistency with experiment, we initiate cascades using primary recoil energies consistent with those initiated by 20.3 MeV $W^{6+}$ ions impacting tungsten, as generated using SRIM. While it is possible to successively introduce individual atomic recoils in a simulation box until a high cumulative dose is reached, this would require a prohibitively long simulation time due to the relatively high probability of occurrence of low energy recoils. Instead, we initialise multiple cascades at once, totaling a dose increment of 0.0002 dpa, chosen as a compromise between computational performance and minimisation of cascade heating[7]. In each cascade iteration, recoil energies are drawn randomly from the list of SRIM-generated recoil energies until their cumulative dose increment approximately corresponds to the target increment. We reject recoil energies below the minimum threshold displacement energy, $E_{\rm d}^{\rm min} = 46\,{\rm eV}$ for this empirical tungsten potential[6], and above the fragmentation energy, $E_{\rm fr} = 100\,{\rm keV}$[8] in tungsten. Starting with the highest drawn recoil energy $E_{\rm R}$ and continuing in order of descending recoil energies, atoms in the system are chosen at random and assigned a randomly-oriented velocity with magnitude corresponding to $v = \sqrt{2E_{\rm R}/m}$. To avoid spurious coincidental cascades, we redraw each randomly chosen recoil atom until it lies outside the exclusion distances of all previously drawn recoil atoms. The exclusion distance is a function of the recoil energies. Considering that a recoil atom with energy $E_{\rm R}$ approximately melts a spherical region of volume[6]

$$V = \frac{4}{3}\pi R^3 \sim \frac{E_{\rm R}}{E_{\rm melt}}\Omega_0, \tag{S3}$$

where $E_{\text{melt}}$ is the energy per atom required to melt the crystal and $\Omega_0$ is the atomic volume, leading to a molten sphere radius of

$$R \sim \left( \frac{3E_{\text{R}}\Omega_0}{4\pi E_{\text{melt}}} \right)^{1/3}, \tag{S4}$$

A randomly chosen recoil atom $i$ should therefore lie at a distance $R_{ij}$ to any other recoil atom $j$ of at least

$$R_{ij} \geq R_i + R_j + R_{\text{buffer}}, \tag{S5}$$

where $R_i$ and $R_j$ are molten sphere radii of atoms $i$ and $j$, respectively, and $R_{\text{buffer}}$ is an additional buffer region of 0.5 nm to ensure a minimum distance of a few lattice spacings for low energy recoils. We use a conservative estimate for the exclusion radius by estimating the melting energy as $E_{\text{melt}} \approx 3k_{\text{B}}T_{\text{melt}}$, neglecting the additional energy cost from the latent heat of fusion[8]. For the chosen dose increment of 0.0002 dpa, we found it was always possible to arrange recoil atoms in a randomly non-overlapping configuration with negligible computational overhead, with the exclusion volume filling ratio averaging about 10 %.

In this work, atoms with a kinetic energy below the tungsten melting energy ($\sim 1.3$ eV[9]) are subjected to a damping force $f_\tau = -m\dot{x}/\tau$, with time constant $\tau = 16.0$ ps, describing kinetic energy loss due to excitation of electrons through slow-moving ions in a crystal environment[10]. Atoms with kinetic energy above 10 eV are subjected to an electronic stopping force consistent with the electronic stopping table of the SRIM[1] software. No damping or stopping is applied to atoms with intermediate energies in an attempt to describe the loss of electronic conductivity in the liquid-like heat spike[10]. After initialising recoil energies into the system, the simulation is propagated for 10 ps which we found sufficient to conclude the recrystallisation phases for the recoil energies considered here. Except for the damping terms, no other thermostats or barostats are applied; simulation cell dimensions are held fixed throughout the propagation.

After the propagation, velocities are set to zero to bring the system temperature to absolute zero after each recrystallisation phase. Next, the potential energy is minimised with respect to atomic coordinates using the method of conjugate gradients. After the relaxation, a second energy minimisation procedure is applied, this time also allowing box dimensions to vary until the prescribed uniaxial stress state is reached. We found that this two-step procedure converged in fewer iterations than a one-step procedure. In principle, the simulation could be performed at finite temperature, for instance by rescaling velocities after each step rather than zeroing them, however, it needs to be considered that a substantial amount of kinetic energy, and therefore temperature, is introduced at the start of each cascade iteration. By equating the damage energy corresponding to a given dose increment of $\delta\phi$ with the kinetic energy of a gas at temperature $\delta T$, the temperature increase can be found as

$$\delta T = \frac{5E_{\text{d}}\delta\phi}{3k_{\text{B}}}. \tag{S6}$$

For a dose increment of $\delta\phi = 0.0002$ with $E_{\text{d}} = 90$ eV for tungsten, the temperature increase is found as $\delta T = 348$ K. This increase in temperature is initially localised to the molten cascade regions, and is therefore not completely comparable to a homogeneous increase in system temperature. Further, as the system is propagated, this temperature is continuously lost due to electron-phonon damping following $T(t) \sim \delta T \exp(-t/\tau)$. For $\tau = 16$ ps, after 10 ps of propagation about half the temperature remains. In conclusion, the temperature

of the simulated system is in the range between 174 K and 348 K. At such temperatures, vacancies in tungsten remain immobile over the time-scale of the simulation, and therefore we consider this simulation setup to be representative of the experiment undertaken at temperature slightly above room temperature.

After each conjugate gradient relaxation of the simulation cell dimensions, the simulation cell vectors are exported to a file. It remains to determine the eigenstrain tensor. Let $\mathbf{A}_\phi$ be a matrix with columns given by the simulation cell vectors at dose $\phi$. This cell matrix may be expressed in terms of the cell matrix of the unirradiated and unstressed system $\mathbf{A}$ through

$$\mathbf{A}_\phi = \mathbf{F}_\phi \mathbf{A}, \tag{S7}$$

where $\mathbf{F}_\phi$ is the deformation gradient tensor at dose $\phi$. Decomposing the deformation gradient tensor into a plastic and elastic contribution $\mathbf{F}_\phi = \mathbf{F}^{\mathrm{p}}_\phi \mathbf{F}^{\mathrm{e}}_\phi$, and recognising that the elastic deformation remains constant during the simulation by external constraint, $\mathbf{F}^{\mathrm{e}}_\phi = \mathbf{F}^{\mathrm{e}}_0$, and therefore $\mathbf{A}_0 = \mathbf{F}^{\mathrm{e}}_0 \mathbf{A}$ and $\mathbf{F}^{\mathrm{p}}_0 = \mathbb{I}$, we arrive at

$$\mathbf{A}_\phi = \mathbf{F}^{\mathrm{p}}_\phi \mathbf{A}_0. \tag{S8}$$

Under the convention that any non-elastic dimensional change is classified as plastic deformation, meaning we do not distinguish between deformation originating from nano-scale defects or slip of the entire crystal, we may express the plastic deformation as a macroscopic eigenstrain $\mathbf{F}^{\mathrm{p}}_\phi = \mathbb{I} + \boldsymbol{\varepsilon}^*_\phi$. Solving for the eigenstrain, we obtain the relation

$$\boldsymbol{\varepsilon}^*_\phi = \mathbf{A}_\phi \mathbf{A}_0^{-1} - \mathbb{I}. \tag{S9}$$

The choice of the simulation box dimensions follows a subtle line of reasoning. In cascade simulation in a cube-shaped tungsten single-crystal with periodic boundary conditions and side lengths of 70 nm, containing 22 million atoms, it was found that interstitials generated by cascades coalesced to form complex dislocation networks and eventually new crystal plane[11,12] at a dose of 0.3 dpa. A similar observation was reported by Wang *et al.*[13], who characterised ion-irradiated tungsten at room temperature using transmission electron microscopy. Dislocations can be represented as boundaries of internal surfaces of point-defect clusters inside the crystal. At athermal irradiation conditions, the formation of the dislocation network is driven by the coalescence of interstitial defects. The area swept out by a dislocation network scales with the total number of interstitials approximately as $A \sim N_{\mathrm{int}}$, just as the total number of interstitials available in the system scales with the number of atoms in the system as $N_{\mathrm{int}} \sim N$. Relating the net area swept out by dislocations to the area of cross-section of a cubic grain $A_{\mathrm{grain}} \sim N^{2/3}$, we see that the area coverage of the network scales with system size as $A/A_{\mathrm{grain}} \sim N^{1/3}$. Depending on the system size $N$, the dislocation content can either cover a fraction of the cross-section $0 < A/A_{\mathrm{grain}} < 1$, form a system-spanning network $A/A_{\mathrm{grain}} \sim 1$, or even form additional crystal planes $A/A_{\mathrm{grain}} > 1$. In conclusion, the formation of the complex, system-spanning dislocation structures observed by Wang *et al.*[13] requires a minimum simulation box size.

The grains in the drawn tungsten wire are strongly elongated along the wire direction, with dimensions of about 50 nm diameter and 1 µm length. At temperatures below which vacancy migration becomes active, self-ion irradiated tungsten is expected to saturate to a vacancy concentration of 0.3 %[6], leading to an equivalent concentration of interstitials, sufficient to form over a dozen new crystal planes lying perpendicular to the elongated grain direction. The eigenstrain arising from new crystal planes is irreversible with respect

to changes in external stress, which further motivates our choice of describing irradiation eigenstrain as irreversible. At the same time, cascade simulations in much smaller simulation boxes would not generate sufficient interstitials to form a plane, instead resulting in microstructures that are not representative of the experimental scenario. We chose system dimensions of $100 \times 100 \times 250$ unit cells, containing 5 million atoms, which enables formation of up to

$$n_{\text{planes}} = \frac{2 n_{\text{x}} n_{\text{y}} n_{\text{z}} c_{\text{vac}}}{n_{\text{x}} n_{\text{y}}} = \frac{2 * 100 * 100 * 250 * 0.003}{100 * 100} = 1.5 \tag{S10}$$

new crystal planes lying perpendicular to the elongated direction. The external stress is applied uniaxially along the elongated direction. We perform cascade simulations to a dose of up to 0.5 dpa under external stress states $\sigma_{\text{zz}}^{\text{ext}}$ ranging from $-1$ GPa to 2 GPa in steps of 0.5 GPa. To obtain a measure of simulation uncertainty, each stress state simulation is repeated five times with a different random seed in an otherwise identical setup. The eigenstrain tensor $\boldsymbol{\varepsilon}_{\phi}^{*}(\sigma_{\text{zz}}^{\text{ext}})$ is extracted for each stress state, with which the surrogate model is parameterised as described in the main article.

### C. Estimating the wire temperature due to beam heating

Most of the kinetic energy of beam ions implanted in the wire is converted to heat energy; in other words, the wire heats up when exposed to the beam. It is difficult to measure the wire temperature directly as, due to its small sample volume, its emitted black-body radiation is too weak to detect by conventional means. Instead, we derived a theoretical estimate of the temperature profile by solving the one-dimensional heat equation. Following that, we also derived an alternative expression for estimating the peak temperature by measuring the load change of a tensioned wire as the beam is turned on, causing heating of the wire and resulting in thermal expansion.

#### *1. Heat conversion efficiency.*

To estimate the heat conversion efficiency, consider first that the entire kinetic energy lost to electronic stopping is rapidly, i.e. without loss, converted into heat via electron-phonon coupling. Of the remaining damage energy $T_{\text{d}}$, only a small portion is expended in the formation of crystal defects. A conservative estimation using the NRT damage formula $N_{\text{d}} = 0.8 T_{\text{d}}/(2E_{\text{d}})$, assuming that the generated defects are Frenkel pairs (FP) with formation energy $E_{\text{FP}}$, yields the fraction of energy lost to defect generation

$$f \lesssim \frac{N_{\text{d}} E_{\text{FP}}}{T_{\text{d}}} = \frac{0.8 E_{\text{FP}}}{2 E_{\text{d}}} = 0.06, \tag{S11}$$

where we substituted values representative for tungsten ($E_{\text{FP}} = 13.5$ eV[14], $E_{\text{d}} = 90$ eV). This estimate represents an upper limit for several reasons: First, the NRT damage formula overestimates the number of Frenkel pairs produced by a factor of about 3 depending on damage energy. A more accurate defect production model, such as the athermal-ecombination-corrected (arc) dpa model[15] which accounts for defect recombination inside the cascade heat-spike, would yield $f \lesssim 0.02$, meaning a heat conversion efficiency of at least 98 %. Second, fewer defects are are produced as microstructural damage is accumulated, approaching

zero new produced defects at high dose[6]. In conclusion, we may assume that most, if not all, of the beam energy is directly converted into heat.

*2. Solving the heat equation.*

Let the thin wire lie along the $z$-coordinate, extending from $z \in [-l/2, l/2]$, with its ends held fixed at ambient temperature $T_0$. As the wire cross-section is small compared to its length, the temperature profile can be described by the one-dimensional heat equation

$$\frac{\partial}{\partial t} u(z,t) = \frac{1}{k} w(z,t) + \frac{\partial^2}{\partial z^2} u(z,t), \tag{S12}$$

where $u(z,t)$ is the temperature profile, $w(z,t)$ is the heat power density introduced by the beam, and $k$ is the thermal conductivity of the wire material. Here, we neglect energy loss through thermal radiation. This approximation is justified at low temperature, as will be shown to be the case here.

Assuming that the beam current is stationary in time, we solve for the steady-state solution where $\frac{\partial}{\partial t} u(z,t) = 0$, leading to the differential equation

$$0 = \frac{1}{k} w(z) + u''(z), \tag{S13}$$

which is solved by the sum of the particular and homogeneous solutions

$$u(z) = a + bz - \frac{1}{k} \int \mathrm{d}z \int \mathrm{d}z \, w(z), \tag{S14}$$

where constants $a$ and $b$ are identified from the boundary conditions.

As the beam is scanned vertically along the wire, and restricted by the beam-limiting aperture, we assume that the heat power density is uniformly distributed over the irradiated wire section:

$$w(z) = \begin{cases} w_0 & -l_{\mathrm{irr}}/2 \leq z \leq l_{\mathrm{irr}}/2 \\ 0 & \text{otherwise.} \end{cases} \tag{S15}$$

Substituting the heat power density and solving for the constants $a$ and $b$ using the boundary conditions, we arrive at the temperature profile

$$u(z) = T_0 + \frac{w_0}{2k} \left[ l_{\mathrm{irr}} \left( z + \frac{l}{2} \right) + \left( z - \frac{l_{\mathrm{irr}}}{2} \right)^2 \Theta \left( z - \frac{l_{\mathrm{irr}}}{2} \right) - \left( z + \frac{l_{\mathrm{irr}}}{2} \right)^2 \Theta \left( z + \frac{l_{\mathrm{irr}}}{2} \right) \right], \tag{S16}$$

where the Heaviside function is defined as $\Theta(x) = 1$ for $x > 0$, and 0 otherwise. The peak temperature of the wire is found at $z = 0$, the centre of the irradiation section:

$$T_{\mathrm{peak}} = u(0) = T_0 + \frac{w_0}{8k} l_{\mathrm{irr}} (2l - l_{\mathrm{irr}}). \tag{S17}$$

It remains to relate the heat power density $w_0$ to the heavy-ion beam parameters. In experiment, the beam intensity is characterised by measuring the current $I_0$ (in units of

nanoampere, or nA) across the wire arising from absorption of the heavy ions. For ions with charge $Q_{\text{ion}} = eZ$ and kinetic energy $E_{\text{ion}}$, we may express the heat power density as

$$w_0 = \frac{E_{\text{ion}} I_0}{Q_{\text{ion}} l_{\text{irr}} \pi R^2}, \tag{S18}$$

where we assumed that the beam energy is homogeneously distributed over the irradiated wire section. This approximation is valid for the thin wire, as the heat is much faster conducted across the wire diameter than across the wire length. Substituting Eq. (S18) into Eq. (S17), we arrive at

$$T_{\text{peak}} = T_0 + \frac{1}{8k} \frac{E_{\text{ion}} I_0}{Q_{\text{ion}}} \left( \frac{2l - l_{\text{irr}}}{\pi R^2} \right). \tag{S19}$$

Substituting the wire geometry constants $L = 15\,\text{mm}$, $l_{\text{irr}} = 4\,\text{mm}$, $R = 8\,\mu\text{m}$, the ion beam constants $Q_{\text{ion}} = 6e$ and $E_{\text{ion}} = 20.3\,\text{MeV}$, and the thermal conductivity for tungsten $k = 1.64 \times 10^{-4}\,\text{W}/\mu\text{m}/\text{K}$, we arrive at

$$T_{\text{peak}} = T_0 + I_0 \cdot 334\,\text{K}/\text{nA}, \tag{S20}$$

where we made use of the $1\,\text{J} = 1\,\text{VAs}$ unit conversion.

The 16-micron diameter wire in this experiment was subjected to beam currents ranging between 0.02 nA to 0.09 nA (note that Fig. 2b in the article shows the current measured by the 102 µm wire), leading to an estimated peak temperature increase between 6 K to 30 K above ambient temperature. The wire temperature remains close to ambient temperature. For tungsten, this is well below the temperature at which vacancies become mobile, or below which thermal creep is expected.

### 3. *Experimental validation*

An independent estimate of the wire temperature can be obtained by measuring the change in wire tension as the beam is turned on. Consider a wire under tension, held at fixed elongation. As the beam is turned on, the wire heats up and expands, resulting in a decrease in tension. From the previously derived temperature profile, we can relate the drop in tension to the peak wire temperature.

The thermal eigenstrain in a wire with temperature profile $u(z)$, relative to the ambient temperature $u_0$, is given by

$$\boldsymbol{\varepsilon}^*(z) = \alpha \left( u(z) - u_0 \right) \cdot \mathbb{I}, \tag{S21}$$

where $\alpha$ is the linear expansion coefficient. The length change of the wire is obtained by integrating the eigenstrain over the length

$$\Delta L = \int_{-L/2}^{L/2} \mathrm{d}z\, \varepsilon^*_{zz}(z) = \frac{\alpha w_0}{24k} \left( 3l^2 l_{\text{irr}} - l_{\text{irr}}^3 \right), \tag{S22}$$

where we substituted the solution for the one-dimensional heat equation (S16). Next, we use the solution for the wire peak temperature (S17) to eliminate the heat power density $w_0$, resulting in

$$\Delta L = \alpha \left( T_{\text{peak}} - T_0 \right) \frac{3l^2 - l_{\text{irr}}^2}{6l - 3l_{\text{irr}}}. \tag{S23}$$

The change in load is determined with Hooke's law

$$\Delta F = -k\Delta l = -\frac{E\pi R^2}{l}\,\Delta l. \tag{S24}$$

Substituting (S23) into the above expression and solving for the peak temperature, we arrive at

$$T_{\text{peak}} = T_0 + \Delta F\,\frac{3L(l_{\text{irr}} - 2l)}{\alpha E\pi R^2(3l^2 - l_{\text{irr}})}. \tag{S25}$$

Substituting the geometric constants for the tungsten wire ($l = 15\,\text{mm}$, $l_{\text{irr}} = 4\,\text{mm}$, $R = 8\,\mu\text{m}$), the linear expansion coefficient $\alpha = 4.3 \times 10^{-6}\,\text{K}^{-1}$, and the Young's modulus ($E = 410\,\text{GPa}$), we arrive at

$$T_{\text{peak}} = T_0 - \Delta F \cdot 5.0\,\text{K/mN}. \tag{S26}$$

In Fig. 2b, it is shown that upon exposure of the sample to a beam current of $I_0 = \frac{16}{102} * 0.2\,\text{nA} = 0.03\,\text{nA}$, the wire tension reduces by approximately 25 MPa, corresponding to a reduction in load of 5 mN. The load reduction suggests an increase in peak temperature of 25 K. The prediction of the peak temperature following Eq. (S20) is 10 K. The temperature cannot be precisely determined using these indirect methods because it is difficult to account for the thermal response of the entire measuring apparatus. In either case, thermal creep is not expected to occur at either of the two estimated temperatures.

## S2. SUPPLEMENTAL INFORMATION TO EXPERIMENTS

### A. Sample material

#### 1. *Potassium-doped tungsten wire*

The drawn potassium-doped tungsten wires with a diameter of 16 µm were manufactured by *ams OSRAM GmbH*, Schwabmünchen (Germany). The manufacturer ensures a weight content of potassium of 75 ppm. The wire is produced out of sintered ingots, of which the chemical composition is reported elsewhere[16]. The wire drawing procedure follows the standard process described for example by Mullendore et al.[17]: The sintered ingots are hot-worked into rods of 2 mm to 4 mm diameter, which is drawn through dies with successively decreasing opening diameters, reducing the diameter with each drawing process. The drawing temperature is decreased alongside the die opening diameter[18]. Although the exact drawing temperatures are not reported, the investigated 16 µm thin wires can be considered a cold-drawn product since its drawing temperature was kept below the recrystallization temperature of tungsten[19].

#### 2. *Sample preparation*

The samples are produced from the aforementioned potassium-doped tungsten wire. To simplify the handling and to ensure that the samples are not damaged, they are glued to polypropylene (PP) frames using a epoxy resin. These frames are laser cut from a 450 µm thick foil and laser engraved with alignment marks as well as a sequential sample number.

For the assembly, a dedicated fixture was designed, with surfaces made out of polytetrafluoroethylene (PTFE) to reduce adhesion of the epoxy resin and dowel pins for precise alignment of the wires. The fixture together with an inserted frame is shown in figure S2. Prior to the first use and then after every 10 frames, all PTFE surfaces were sealed using *Mold Sealer S-31*. In addition, the release agent *Treil Part 310* is used before each application. Both primers are manufactured by *Jost Chemicals GmbH* and additionally help to reduce the adhesion of the frame to the PTFE.

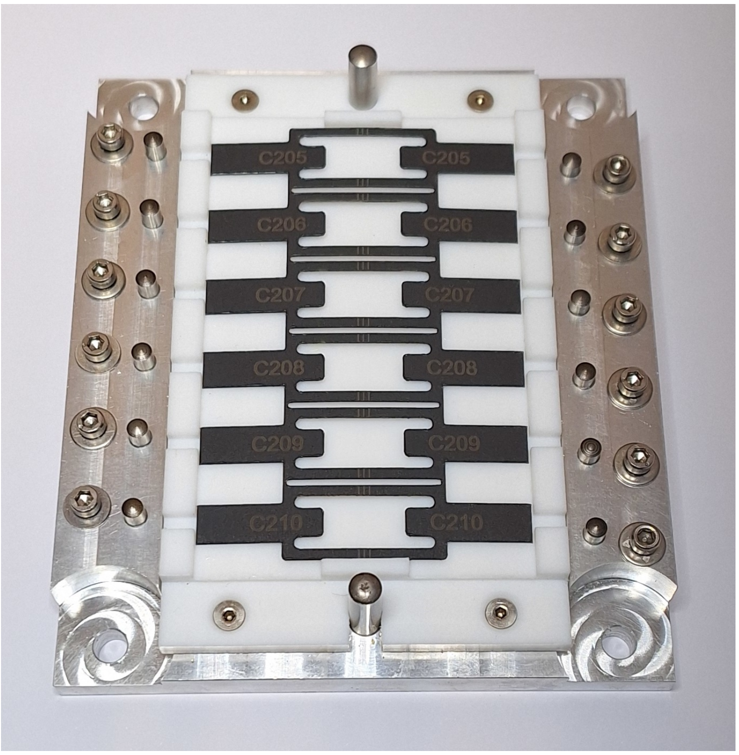


**Fig. S2:** Sample fixture with inserted frame. 6 samples can be prepared simultaneously.

For the assembly, first one of the frames is placed in the mounting fixture and then for each of the 6 positions a 120 mm long piece of wire is clamped over the sample frame using screws. It is important to ensure that the wire is not additionally tensioned by tightening the screws. Ideally, the wire should only be tensioned to the extent that it no longer sags, which can be easily checked by the reflection of a light source on the wire surface. A very small amount of epoxy resin *UHU PLUS ENDFEST 300* is then applied to both ends. A spot of about 3 mm by 1 mm is sufficient. A PTFE counter plate followed by an aluminum plate for load distribution is placed on top and clamped using two screw clamps. After 24 hours of curing time, the frame with the glued-on wires can be removed from the mounting device and divided into individual samples.

In order to contact the samples electrically, a copper tape is wrapped around the end of the frame. After one revolution, the protruding wire is folded onto the copper surface and wrapped again with the copper tape. This process is repeated for the second half and the excess wire ends are cut off. The electrical continuity through the samples is then tested using a multimeter. Samples without continuity or with a resistance greater than 35 Ω are rejected. The free length of the finished glued-in samples is 15 mm. Figure S3 shows a complete sample.

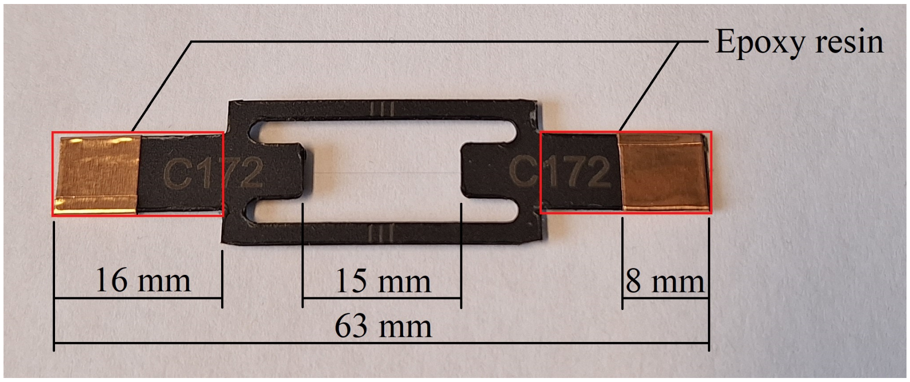


**Fig. S3:** Complete sample with copper tape at both ends to facilitate electrical contacting

## B. The GIRAFFE Experiment

The **G**eneral-Purpose **Irra**diated **F**iber and **F**oil **E**xperiment (GIRAFFE) is an experimental facility located at the tandem accelerator laboratory of the Max Planck Institute for Plasma Physics. This experiment was specifically designed to investigate the synergistic effects of different extreme conditions on materials, especially in the realm of fusion research. The high-energy ion beam of a particle accelerator can be used to generate dislocation damage that simulates the damage caused by neutron irradiation. In addition a plasma source provides low-energy ions such as deuterium (D) or helium (He), which can be used to mimic the particle flux in a fusion reactor. The sample can also be simultaneously tensioned, which is suitable for simulating a mechanical load as well as for mechanically testing the sample. As a further analysis method, a built-in set of two detectors can be used for Nuclear Reaction Analysis (NRA) as well as Rutherford Backscattering Spectroscopy (RBS). The individual loadings, as well as the analysis, can be carried out *in situ* without exposing the sample to the atmosphere between the different steps.

### *1. Tandem accelerator*

The high-energy ion beam is generated by a 3 MV *Tandetron* tandem accelerator from *High Voltage Engineering*[20]. The tungsten ions, used in this work, are generated as $W^-$ in a caesium sputter source *Model 860C* from *High Voltage Engineering*. The negative ions are accelerated towards the positive high voltage terminal at 2900 kV, where a stripper gas is used to change the charge to $W^{6+}$. The now positive ions are further accelerated in the second half of the acceleration path and focused at the end via an electrostatic quadrupole triplet. To ensure a homogeneous irradiation along the sample axis, the beam is scanned over the sample using an electrostatic scanning system with a frequency of 1 kHz. The kinetic energy of the ions ($E_\mathrm{i}$) at the end of the tandem acceleration is calculated according to equation S27 using the charge state ($Z$), the terminal voltage ($U_\mathrm{T}$) and the elementary charge ($e$):

$$E_\mathrm{i} = (Z + 1)\, U_\mathrm{T}\, e. \tag{S27}$$

This results for the $W^{6+}$ ions in this work in an energy of 20.3 MeV, see equation S28:

$$E_{\mathrm{W}^{6+}} = (6 + 1) \cdot 2.9\,\mathrm{MV} \cdot e = 20.3\,\mathrm{MeV}. \tag{S28}$$

To determine the ion fluence $\Phi$ on the sample, the electric current flowing over the sample to ground is measured. For this purpose, one of the sample ends is connected to a *Keithley 6487* picoamperemeter, with the measuring range set to 2 nA and a sampling time of 200 ms. According to equation S29, the fluence can then be calculated from the measured current $I$ and the projected sample surface $A_{\text{irr}}$ as seen by the ion beam:

$$\Phi(t) = \frac{1}{eZA_{\text{irr}}} \int_{t_0}^{t} I(t')\,\mathrm{d}t' \tag{S29}$$

The sample surface emits secondary electrons when it is impacted by the high-energy ions, leading to an additional electric current flowing across the sample, thus affecting the fluence measurement. A similar effect occurs when the beam hits one of the beam limiting apertures; the secondary electrons emitted there can also reach the sample and influence the measurement result. To reduce the measurement error resulting from secondary electron emission, the sample is enclosed by two shielding electrodes charged to −500 V during the experiment. The resulting electric field repels the secondary electrons back to their origin. Figure S4 shows the schematic measurement setup including the electrical connections.

#### *2. Experiment preparation*

After mounting the sample, the distance between the two sample holders is reduced using a *PiezoMotor LTC300* linear piezo motor to ensure that the sample is not under tensile stress. The two longitudinal strips of the sample frame are then cut using a diagonal cutter, so that the sample is free between the two holders. To ensure a uniaxial load during the experiment, the sample is preloaded with 50 mN and the upper sample holder is moved alternately in both axes perpendicular to the wire using an x-y table until a load minimum is reached.

An additional measuring electrode made of a 102 µm diameter tungsten wire is attached to the lower sample holder. The entire measurement setup can be rotated along the sample axis, allowing the measuring wire to be positioned either in front of or behind the sample. At the beginning of the experiment, the measuring electrode is positioned in front of the sample so that, while the ion beam is adjusted, the sample lies in the beam shadow and is not yet irradiated. After all adjustments have been completed, the measuring electrode is rotated by 180° so that it is positioned exactly behind the sample. Both the sample and the measuring electrode are at the same electrical potential, which means that both signals are added together in the ion current measurement. This is necessary because the signal to noise ratio of a single 16 µm sample is not precise enough. The entire test setup is then installed in a vacuum chamber on one of the 10° beamlines of the tandem accelerator and evacuated until a pressure of about $10^{-6}$ mbar is reached.

### C. Irradiation-induced stress relaxation

#### *1. Post-irradiation analysis*

An irradiated sample was investigated using scanning electron microscopy (SEM) in order to detect any beam-induced changes in the wire's microstructure. For this purpose, the wire was first coated with a thin layer of Pt in order to improve its handling. For this, the

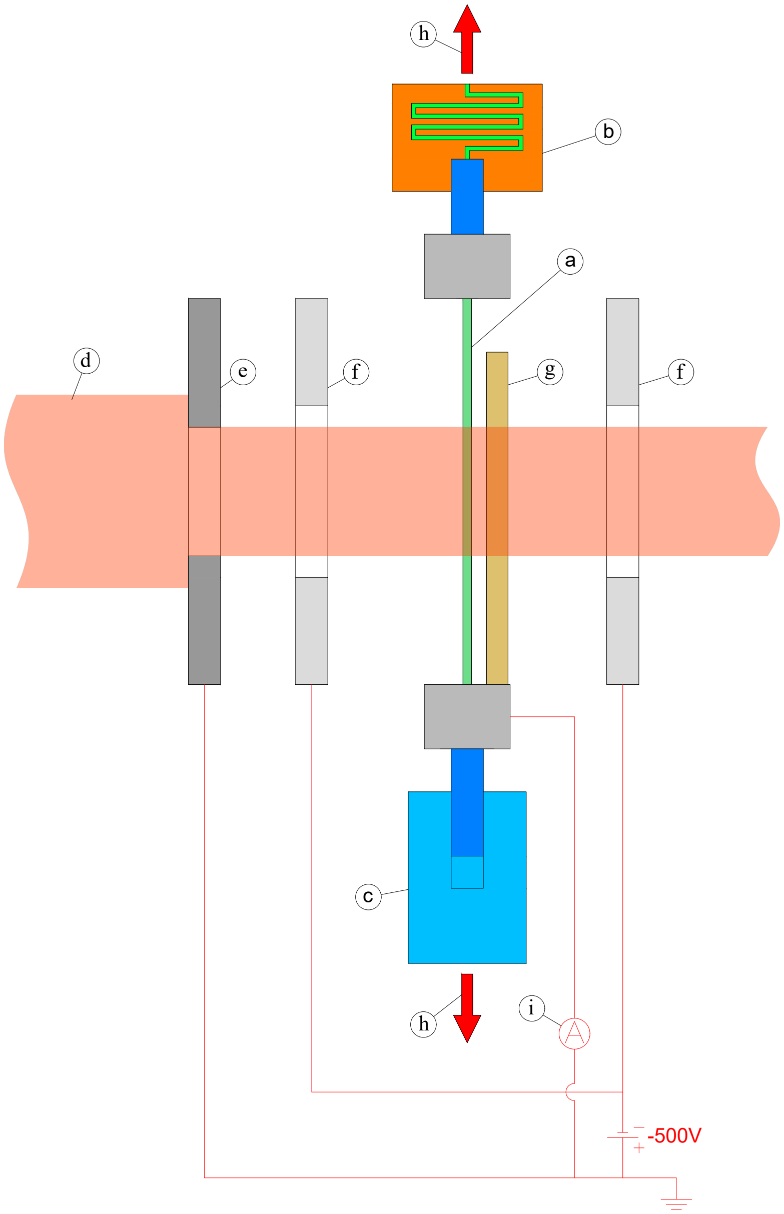


**Fig. S4:** Schematic view of the current measurement setup:
(a) 16 µm sample; (b) load cell; (c) linear piezo motor; (d) high-energy ion beam; (e) beam limiting aperture; (f) suppressing electrodes; (g) 102 µm measuring wire; (h) tensile force; (i) picoamperemeter

irradiated section of the wire was glued across a hole punched into a Kapton foil. Then, it was immersed into a beaker filled with *Jentner® Platinum Bath JE18™*. By applying a voltage of 1.7 V between the sample and a counter-electrode, the irradiated wire section was coated with a homogeneous layer of platinum. Electroplating for a duration of 30 min resulted in a radial thickness of the platinum layer of $(6.1 \pm 0.3)$ µm yielding a sample thickness of around 30 µm. The coated wire was then glued to an Al support using conductive Ag paint and Cu tape in order to prepare them for the FIB cross-sectioning routine. Cross-sectioning

was performed using a *ThermoFisher FEI Helios NanoLab 600* FIB-SEM equipped with a focused $Ga^+$ ion beam. Prior to cross-sectioning, the sample surface was coated with a thin layer of Pt by means of *in situ* ion beam assisted metal deposition in order to avoid uneven sputtering during cross-sectioning. Coarse cuts were performed using a beam current of 21 nA. In order to improve the sample surface, a lower beam current as low as 0.46 nA was used subsequently. The acceleration voltage was 30 kV throughout the FIB preparation process.

The microstructure of the irradiated sample was imaged using secondary electron contrast at eight different positions on the wire cross-section. The positions of the SE images can be described in polar coordinates by $(r, \phi) = (0.85\,R, j \cdot 45°)$, where $j = 1 \ldots 8$ is the number of the image and $R$ is the wire radius. In this way, the microstructure of the irradiated wire could be quantified along its circumference. The grain size in each SE image was determined using the line-intersection method. The results are shown in figure S5. The diagram clearly shows, that the mean grain size is comparable along the whole wire circumference. Using the fitted logarithmic normal distributions, the mean grain size in each image can be calculated. Averaging over all images, the mean size of grains viewed along the wire axis is $(106 \pm 9)$ nm. This lines up well with the result of $(113 \pm 13)$ nm which was determined from the as-received wire using the same method. Thus, there is no evidence of any irradiation-induced recrystallization or any other significant change in the microstructure. Hence, it is concluded that the observed effect of stress-relaxation is not an artefact of grain restoration.

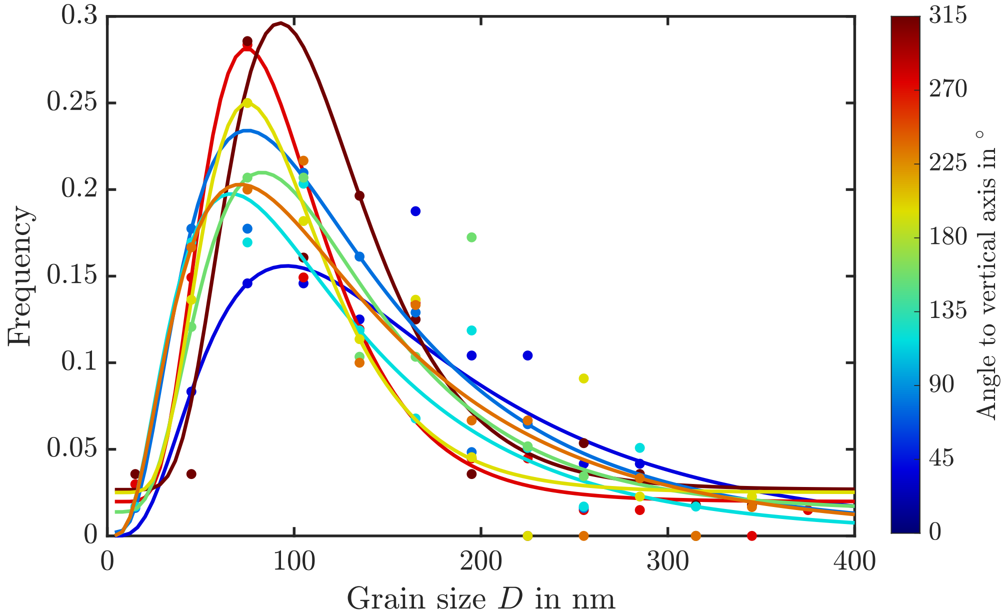


**Fig. S5:** Distribution of grain sizes $D$ at different positions in the vicinity of the wire surface. The measurements were taken at different azimuthal positions with a constant distance to the wire centre. The azimuthal angle (with respect to an arbitrary vertical axis) is colour-coded (see colorbar to the right side of the figure). The solid lines represent fitted logarithmic normal distributions.


* max.boleininger@ukaea.uk

[1] J. F. Ziegler, Nuclear Instruments and Methods in Physics Research Section B: Beam Interactions with Materials and Atoms **219**, 1027 (2004).

[2] R. E. Stoller, M. B. Toloczko, G. S. Was, A. G. Certain, S. Dwaraknath, and F. A. Garner, Nuclear instruments and methods in physics research section B: beam interactions with materials and atoms **310**, 75 (2013).

[3] R. E. Stoller, M. B. Toloczko, G. S. Was, A. G. Certain, S. Dwaraknath, and F. A. Garner, Nuclear Instruments and Methods in Physics Research Section B: Beam Interactions with Materials and Atoms **459**, 196 (2019).

[4] A. Y. Konobeyev, U. Fischer, Y. A. Korovin, and S. P. Simakov, Nuclear Energy and Technology **3**, 169 (2017).

[5] M. J. Norgett, M. T. Robinson, and I. M. Torrens, Nuclear Engineering and Design **33**, 50 (1975).

[6] M. Boleininger, D. R. Mason, A. E. Sand, and S. L. Dudarev, Scientific Reports **13**, 1684 (2023).

[7] G. Vineyard, Radiation effects **29**, 245 (1976).

[8] A. De Backer, A. E. Sand, K. Nordlund, L. Luneville, D. Simeone, and S. L. Dudarev, EPL (Europhysics Letters) **115**, 26001 (2016).

[9] For the sake of physical accuracy, we use here the more accurate estimate which includes the latent heat of fusion.

[10] D. R. Mason, Journal of Physics: Condensed Matter **27**, 145401 (2015).

[11] D. R. Mason, S. Das, P. M. Derlet, S. L. Dudarev, A. J. London, H. Yu, N. W. Phillips, D. Yang, K. Mizohata, R. Xu, and F. Hofmann, Physical Review Letters **125**, 225503 (2020).

[12] M. Boleininger, S. L. Dudarev, D. R. Mason, and E. Martínez, Physical Review Materials **6**, 063601 (2022).

[13] S. Wang, W. Guo, T. Schwarz-Selinger, Y. Yuan, L. Ge, L. Cheng, X. Zhang, X. Cao, E. Fu, and G.-H. Lu, Acta Materialia **244**, 118578 (2023).

[14] P.-W. Ma and S. L. Dudarev, Phys. Rev. Materials **3**, 063601 (2019).

[15] K. Nordlund, S. J. Zinkle, A. E. Sand, F. Granberg, R. S. Averback, R. Stoller, T. Suzudo, L. Malerba, F. Banhart, W. J. Weber, *et al.*, Nature Communications **9**, 1 (2018).

[16] M. Fuhr, T. Höschen, J. Riesch, M. Boleininger, J. Almanstötter, W. Pantleon, and R. Neu, Philosophical Magazine **103**, 1029 (2023).

[17] J. A. Mullendore, in *The Metallurgy of Doped/Non-Sag Tungsten*, edited by E. Pink and L. Bartha (Elsevier Applied Science, Essex, 1989) pp. 61–82.

[18] S. W. Yih and C. T. Wang, *Tungsten: Sources, Metallurgy, Properties and Applications* (Plenum Press, New York and London, 1979).

[19] G. W. Meetham and M. H. van de Voorde, in *Materials for High Temperature Engineering Applications*, edited by G. W. Meetham and M. H. van de Voorde (Springer Berlin Heidelberg, Berlin, Heidelberg, 2000) pp. 86–89.

[20] D. Mous, R. Koudijs, P. Dubbelman, and H. van Oosterhout, Nuclear Instruments and Methods in Physics Research Section B: Beam Interactions with Materials and Atoms **62**, 421 (1992).
